# Supplementary material for: Ab initio molecular dynamics study of dissociation of water under an electric field
Source: arXiv:1204.1120 source file (2012-04-05)
Supplement: Supplementary file 1 [file supplem_inf_prl.pdf]

# Auxiliary information for "*Ab initio* molecular dynamics study of dissociation of water under an electric field"

A. Marco Saitta[1] [†], Franz Saija[2] [*], Paolo V. Giaquinta[3] [‡]
[1] *IMPMC, CNRS-UMR 7590, Université P & M Curie, 75252 Paris, France*
[2] *CNR-IPCF, Viale Ferdinando Stagno d'Alcontres 37, 98158 Messina, Italy*
[3] *Università degli Studi di Messina, Dipartimento di Fisica, Contrada Papardo, 98166 Messina, Italy*

Our system contained 64 water molecules, twice as large as the one employed by Geissler and coworkers [4], and was thus sufficiently big to combine quantum-mechanical accuracy with the typical length scales of the problem. Molecules were arranged in a cubic box of 12.4 Å side, corresponding to ambient density. Oxygen and hydrogen electron-ion interactions were modeled by ultrasoft pseudopotentials within the DFT-PBE functional, with a kinetic energy cutoff of 25 Ry for the wavefunctions and 200 Ry for the charge density. We counterchecked our results through dissociation tests with cutoffs of 50 Ry/400 Ry respectively, obtaining very similar results. Brillouin zone integrations were performed at the Γ point.

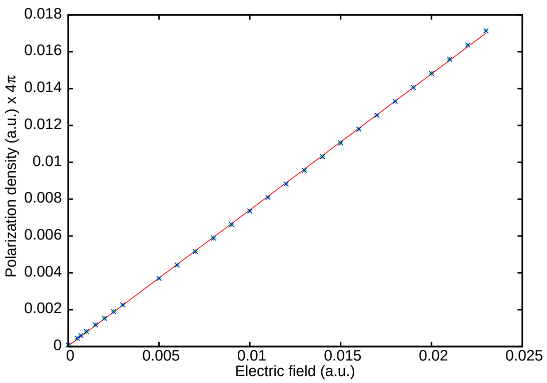


FIG. 1: Field-induced variation of the electronic polarization plotted as a function of the external field, calculated at fixed ionic positions as in Ref. [1]. The crosses represent the calculated points, while the straight line is a linear fit, yielding a high-frequency dielectric constant of 1.74.

We employed the Berry theory approach to the description of an external electric field as developed in Ref. [1], and recently implemented in the density-functional-based *Quantum Espresso* code [2]. We checked the validity of a finite-field approach by calculating the high-frequency dielectric constant of water as $\epsilon_\infty = 1 + \frac{4\pi}{\Omega} \cdot \frac{\Delta P(E)}{E}$, where $\Omega$ is the volume, $E$ is the electric field intensity, and $\Delta P(E)$ is the field-induced polarization. We report in Fig. 1 the calculated values – for standard neutral configurations of water – of the term $\frac{4\pi\Delta P}{\Omega}$ as a function of the external field. A linear response behavior is observed, at least for values of $E$ up to 0.02 a.u. $\approx$ 1 V/Å. The slope fits to 0.74, which yields $\epsilon_\infty = 1.74$, in good agreement with the experimental value (1.8), as well as with the value (1.72) calculated with *ab initio* methods in [3]. The potentially most dangerous drawback of the method we used may be a field-induced metallization of the system. To check this aspect, we calculated the band structure of the system for several relevant configurations and, in particular, for those corresponding to states just before, during, and soon after a proton jump, and always found safely insulating bandgaps (larger than 3.5 eV).

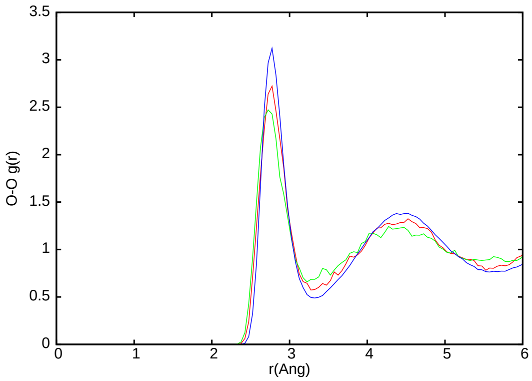


FIG. 2: Oxygen-oxygen pair distribution function calculated at zero field (red line), at a field of 0.15V/Å(green line), and in fieldless CP calculations at 323 K and using a BLYP functional (blue line).

The system evolved in time through a Car-Parrinello (CP) dynamics, with a fictitious electronic mass of 300 *a.u.* and a timestep of 0.096 *fs* over trajectories of the order of a few picoseconds, for each value of the external electric field. Most simulations were performed at a nominal temperature of 350 K, but tests at 300 K and 250 K confirmed the molecular dissociation to take place for the same values of the external field. Although the dynamics of the nuclei was completely classical, we checked the effect of the mass in deuterated water, finding again very similar results, *i.e.* molecular dissociation for a field intensity of 0.35 V/Å. We report in Fig. 2 the oxygen-oxygen pair distribution function, calculated at T=350 K for zero field and for a field of 0.15 V/Å, and compared with similar CP calculations carried out at a lower temperature (323 K) and with a different functional (BLYP). To better illustrate the effect of the field on bulk water before dissociation, we report in Fig. 3 the molecular polar angle distribution with respect to the direction of a field of intensity 0.15 V/Å. We finally report in Fig. 4 the instantaneous count of net positive charges (*i.e.* proton

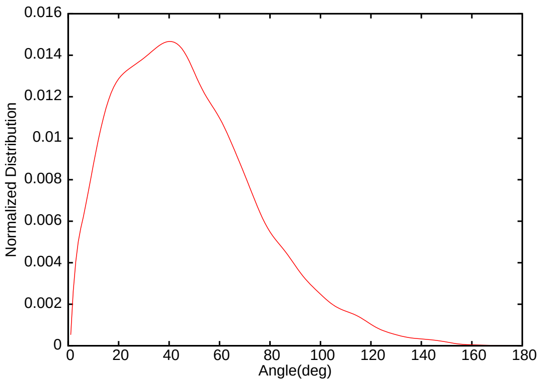


FIG. 3: Distribution of the instantaneous angles formed by the axis of water molecules with respect to the direction of the field for an intensity of 0.15 V/Å.

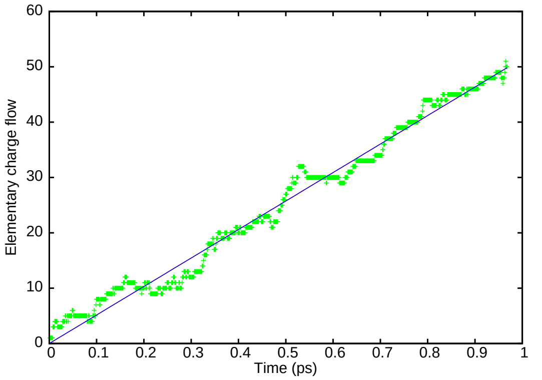


FIG. 4: Number of net charges (green crosses) traversing a section of the simulation cell along a direction parallel to the field plotted as a function of time, for a field intensity of 1.0 V/Å. The blue line is a linear fit yielding the current intensity.

minus hydroxide ions) transversing a section of the unit cell perpendicular to the field as a function of time, for a field intensity of 1.0 V/Å, which allowed us to obtain the current intensity and the associated resistivity.

[†] Corresponding author. E-mail: `marco.saitta@impmc.upmc.fr`
[*] E-mail: `saija@me.cnr.it`
[‡] E-mail: `paolo.giaquinta@unime.it`
[1] P. Umari, A. Pasquarello, *Phys. Rev. Lett.* **89**, 157602 (2002).
[2] P. Giannozzi *et al.*, *J. Phys. Condens. Matter* **39**, 395502 (2009).
[3] Y. Lu, F. Gygi, G. Galli, *Phys. Rev. Lett.* **100**, 147601 (2008).
[4] P. L. Geissler, C. Dellago, D. Chandler, J. Hutter, M. Parrinello, *Science* **291**, 2121 (2001).
